# Supplementary material for: Electromagnetically induced moir\'{e} optical lattices in a coherent atomic gas
Source: arXiv:2202.11275 source file (2022-02-23)
Supplement: Supplementary file 1 [file Supplementary_Information_for_FOP_2021_0288_R1.tex]

%\documentclass[aps,pra,preprint,groupedaddress,amsmath,amssymb,showpacs,10pt,twocolumn]{revtex4-1}
%\usepackage{graphicx,mathrsfs,epsfig,epstopdf,amsmath,amssymb,multirow}
%\usepackage[colorlinks,	linkcolor=blue,anchorcolor=blue,citecolor=blue,bookmarksnumbered]{hyperref}
%\usepackage{dcolumn}% Align table columns on decimal point
%\usepackage{bm}
%\allowdisplaybreaks
\documentclass[pra,showpacs,superscriptaddress,10pt,amsmath,amssymb]{revtex4-1}
\usepackage[colorlinks,citecolor=blue,linkcolor=red,dvipdfm]{hyperref}
\usepackage{amsmath,amssymb,graphicx}
\usepackage{caption}
\usepackage{times}
\usepackage{float}
%%%%%%%%%%%%%%%%%%%%%%% begin %%%%%%%%%%%%%%%%%%%%%%%%%%%%%%twocolumn,

\begin{document}

\title{Supplementary Information for ``Electromagnetically induced moir\'{e} optical lattices in a coherent atomic gas"}

\author{Zhiming Chen}
\affiliation{State Key Laboratory of Transient Optics and Photonics, Xi'an
Institute of Optics and Precision Mechanics of Chinese Academy of Sciences, Xi'an 710119, China}
\affiliation{School of Science, East China University of Technology, Nanchang 330013, China}
\affiliation{Collaborative Innovation Center of Light Manipulations and Applications, Shandong Normal University, Jinan 250358, China}

\author{Xiuye Liu}
\affiliation{State Key Laboratory of Transient Optics and Photonics, Xi'an
Institute of Optics and Precision Mechanics of Chinese Academy of Sciences, Xi'an 710119, China}
\affiliation{University of Chinese Academy of Sciences, Beijing 100049, China}

\author{Jianhua Zeng}
\email{\underline{zengjh@opt.ac.cn}}
\affiliation{State Key Laboratory of Transient Optics and Photonics, Xi'an
Institute of Optics and Precision Mechanics of Chinese Academy of Sciences, Xi'an 710119, China}
\affiliation{University of Chinese Academy of Sciences, Beijing 100049, China}
\begin{abstract}
This supplementary documents provide further details on deriving the envelope equation that governs the fundamental theory of creating electromagnetically induced moir\'{e} optical lattices in the main text. In Sec.~\ref{Sec:1}, we describe the physical model under consider and give the explicit expressions of the underlying Maxwell-Bloch equations. We show the derivation of the two-dimensional envelope equation in Sec.~\ref{Sec:2}.
\end{abstract}
\date{\today}
\maketitle

\captionsetup[figure]{labelfont={bf},labelformat={default},labelsep=period,name={Fig.}}

\section{ Maxwell-Bloch equations}{\label{Sec:1}}

We consider light propagation in a three-level $\Lambda$-type coherent atomic ensemble that is cooled to an ultralow temperature to eliminate the Doppler broadening effect~\cite{EIT-OL2d} [See Fig. 1(a) in the main text]. A weak probe field with half-Rabi frequency $\Omega_p$ and center angular frequency $\omega_p$ couples ground state $|1\rangle$ to excite state $|3\rangle$, and a very strong continuous-wave control field with half-Rabi frequency $\Omega_c$ and center angular frequency $\omega_c$, modulated periodically in spatial, bridges metastable state $|2\rangle$ to excite state $|3\rangle$. The spontaneous emission decay rates of transitions $|3\rangle \rightarrow |1\rangle$ and $|3\rangle \rightarrow |2\rangle$ are represented by $\Gamma_{13}$ and $\Gamma_{23}$, and the detunings $\Delta_2=\omega_{p}-\omega_{c}-\omega_{21}$ and $\Delta_3=\omega_{p}-\omega_{31}$, here $\omega_{jl}=(E_j-E_l)/\hbar$ with $E_j$ being the eigen energy of state $|j\rangle$. It should be noted that, in reality, the energy levels $|1\rangle$, $|2\rangle$, and $|3\rangle$ can be selected respectively as $5^{2}\textrm{S}_{1/2}(F=1)$, $5^{2}\textrm{S}_{1/2}(F=2)$, and $5^{2}\textrm{P}_{1/2}(F=2)$ states of $^{87}$Rb atoms tuned to D1-line transition~\cite{Steck}. Under an appropriate condition, the two laser fields and the atomic gas result in a well-known EIT core where the absorption of the probe field can be suppressed remarkably due to the quantum interference effect induced by the control field~\cite{FIM}. To obtain the electromagnetically induced moir\'{e} optical lattices under the EIT condition, the control field (after simplification) is chosen as the periodic function of spatial coordinates $(x,\,y)$ [See the main text].

In our model, both the probe and control laser fields are assumed to propagate along the $z$ direction, thus the electric-field vector can be written as $\textbf{E}=\textbf{E}_p+\textbf{E}_c=\hat{\mathbf{e}}_{p}{\cal E}_{p} e^{i(k_{p} z-\omega_{p} t)}+\hat{\mathbf{e}}_{c}{\cal E}_{c}(x,y) e^{i(k_{c} z-\omega_{c} t)}+\textrm{c.c.}$. Here $\hat{\mathbf{e}}_{p}$ ($\hat{\mathbf{e}}_{c}$) is the unit vector of the probe (control) field with the envelope ${\cal E}_p$ (${\cal E}_c$), $\omega_p$ ($\omega_c$) is the angular frequency of the probe (control) field, and $k_{p}=\omega_{p}/c$ ($k_c=\omega_c/c$) is the wavenumber of the probe (control) field before entering the atomic gas.
%%Additionally, to implement in the form of electromagnetically induced Moir\'{e} lattice, we set the control field is the function of spatial coordinates (i.e., $x,\,y$).
%
Under the methods of electric-dipole and rotating-wave approximations, the Hamiltonian of the system in the interaction picture is
%\begin{eqnarray}
$$\hat{\cal H}_{\rm int}=-\sum_{j=1}^{3}\hbar\Delta_j|j\rangle\langle j|-\hbar\,\left[\Omega_c|3\rangle\langle2|+\Omega_{p}|3\rangle\langle1|+{\rm H.c.}\right],\eqno{(\textrm{S1})}$$ {\color{red}with $\Delta_1=0$}.
%\end{eqnarray}
Here $\Omega_c=(\mathbf{p}_{23}\cdot{\hat{\mathbf {e}}}_c){\cal E}_c/\hbar$ and $\Omega_{p}=(\mathbf{p}_{13}\cdot{\hat{\mathbf {e}}}_{p}){\cal E}_{p}/\hbar$ are half Rabi frequencies of the control and probe fields, where $\textbf{p}_{jl}$ is the electric dipole matrix element related to the transition from $|j\rangle$ to $|l\rangle$.
Thus the equation of motion for density matrix $\sigma$ in the interaction picture is given by
%%
%\begin{subequations}\label{dme}
%\begin{eqnarray}
$$i\frac{\partial}{\partial
t}\sigma_{11}-i\Gamma_{13}\sigma_{33}+\Omega_p^{\ast}\sigma_{31}-\Omega_p\sigma_{31}^{\ast}=0, \eqno{(\textrm{S2a})}$$
$$i\frac{\partial}{\partial
t}\sigma_{22}-i\Gamma_{23}\sigma_{33}+\Omega_{c}^{\ast}\sigma_{32}-\Omega_{c}\sigma_{32}^{\ast}=0, \eqno{(\textrm{S2b})}$$
$$i\frac{\partial}{\partial
t}\sigma_{33}+i(\Gamma_{13}+\Gamma_{23})\sigma_{33}-\Omega_p^{\ast}\sigma_{31}+\Omega_p\sigma_{31}^{\ast}\-\Omega_c^{\ast}\sigma_{32}+\Omega_c\sigma_{32}^{\ast}=0, \eqno{(\textrm{S2c})}$$
$$\left(i\frac{\partial}{\partial
t}+d_{21}\right)\sigma_{21}-\Omega_p\sigma_{32}^{\ast}+\Omega_c^{\ast}\sigma_{31}=0,\eqno{(\textrm{S2d})}$$
$$\left(i\frac{\partial}{\partial
t}+d_{31}\right)\sigma_{31}-\Omega_p(\sigma_{33}-\sigma_{11})+\Omega_c\sigma_{21}=0,\eqno{(\textrm{S2e})}$$
$$\left(i\frac{\partial}{\partial
t}+d_{32}\right)\sigma_{32}-\Omega_c(\sigma_{33}-\sigma_{22})+\Omega_p\sigma_{21}^{\ast}=0,\eqno{(\textrm{S2f})}$$
%\end{eqnarray}
%\end{subequations}
%%
where $d_{jl}=\Delta_{j}-\Delta_{l}+i\gamma_{jl}$.
Dephasing rates are defined as
$\gamma_{jl}=(\Gamma_j+\Gamma_l)/2+\gamma_{jl}^{\rm col}$ with
$\Gamma_j=\sum_{E_i<E_j}\Gamma_{ij}$  being the spontaneous
emission rate from the state $|j\rangle$ to all lower energy
states $|i\rangle$ and $\gamma_{jl}^{\rm col}$  being the
dephasing rate reflecting the loss of phase coherence between
$|j\rangle$ and $|l\rangle$.

According to the method of slowly varying envelope approximation, the Maxwell equation for the probe-field Rabi frequency $\Omega_{p}$ is described as~\cite{QHH}
%%%
%\begin{eqnarray}\label{ME}
$$i\left(\frac{\partial}{\partial
z}+\frac{1}{c}\frac{\partial}{\partial t}\right)\Omega_{p}+\frac{c}{2\omega_{p}}\left(\frac{\partial^2 }{\partial x^2}+\frac{\partial^2}{\partial y^2}\right)\Omega_{p}+\frac{\omega_{p}}{2c}\chi_p\Omega_{p}=0, \eqno{(\textrm{S3})}$$
%\end{eqnarray}
%%%
where $\chi_p={\cal N}_a|\mathbf{p}_{13}\cdot \hat{\mathbf{e}}_{p}|^2\sigma_{31}/(\hbar\varepsilon_0 \Omega_{p})$ is the optical susceptibility of the probe field, with ${\cal N}_a$ being atomic density. Because we focus on the stationary state of the system under study, we assume that the time duration of the probe field is very large, i.e., the time derivatives in the Maxwell-Bloch Eqs. (S2) and (S3) can be neglected appropriately.
%which is valid for the probe field with a longer time duration.
%%%%%%%%%%%%%%%%%%%%%%%%%%%%%%%%%%%%%%%%%%%%%%%%%%%%%%%%%%%%%%%%%%%%%%%%%%%%%%%%%%
%
\section{Derivation of envelope equation}{\label{Sec:2}}
To investigate electromagnetically induced moir\'{e} optical lattices in the linear circumstance, we assume that the intensity of probe field is very weak. Thus the Bloch Eq. (S2) can be solved by using a perturbation expansion, i.e., $\Omega_p$ being taken as a small parameter. The linear solution of nondiagonal element is read as
%\begin{eqnarray}
$$\sigma_{31}=\frac{d_{21}\Omega_p}{|\Omega_c|^2-d_{21}d_{31}}. \eqno{(\textrm{S4})}$$
%\end{eqnarray}
Based on this solution we can achieve the expression of the optically induced susceptibility of the probe field with the form~\cite{ZLM,ZWZ}
%%%
%\begin{eqnarray}
$$\chi_p=\frac{{\cal N}_a|\mathbf{p}_{13}\cdot \hat{\mathbf{e}}_{p}|^2}{\hbar\varepsilon_0}\frac{d_{21}}{|\Omega_c|^2-d_{21}d_{31}}. \eqno{(\textrm{S5})}$$
%\end{eqnarray}
%%
%

Because of the energy levels being selected from $^{87}$Rb atoms tuned to D1-line transition, the decay rates are given by $\Gamma_2\simeq 1.0$ kHz, and $\Gamma_3\simeq 5.75$ MHz, and $\textbf{p}_{13}=2.54\times10^{-27}$ C cm~\cite{Steck}. Through choosing other parameters $\mathcal{N}_a=3.69\times10^{10}\,V_0$ cm$^{-3}$ ($V_0$ is a real constant), $\Omega_{c0}=1.0\times10^{7}$ Hz, $R=36$ $\mu$m, $\Delta_1=0$, $\Delta_2=1.0\times 10^5$ Hz, and $\Delta_3=1.0\times 10^4$ Hz, the real part and the imaginary part of product term $d_{21}d_{31}$ are much smaller than $|\Omega_{c0}|^2$. In addition, we introduce some dimensionless variables: spatial coordinates $\mathbf{r}=(\xi,\,\eta)=(x,\,y)/R$, $u=\Omega_p/U_0$, and propagation distance $s=z/L_{\rm Diff}$ with typical diffraction length $L_{\rm Diff}=\omega_pR^2/c$. Here $U_0$ and $R$ are the typical Rabi frequency and beam radius of the probe field. Based on the parameters mentioned above, we can obtain the typical diffraction length $L_{\rm Diff}=1.0$ cm. Then the Maxwell equation for the probe-field Rabi frequency can be convert into the dimensionless 2D envelope equation
%\begin{eqnarray}\label{EE}
$$i\frac{\partial u}{\partial
s}=-\frac{1}{2}\left(\frac{\partial^2 }{\partial \xi^2}+\frac{\partial^2}{\partial \eta^2}\right)u
+V_{\mathrm{OL}}(\mathbf{r})u, \eqno{(\textrm{S6})}$$
%\end{eqnarray}
The coefficient of the last term in Eq. (S6) represents the induced moir\'{e} optical lattice potential with lattice depth $V_0$
%%
%\begin{eqnarray}\label{V}
%&&V(\xi,\eta)=\frac{{\cal N}_a|\mathbf{p}_{13}\cdot \hat{\mathbf{e}}_{p}|^2 \omega_p L_{\rm Diff}}{2\hbar\varepsilon_0 c}\frac{d_{21}}{|\Omega_c(\xi,\eta)|^2-d_{21}d_{31}}.
%\end{eqnarray}
%%
%\begin{equation}
%V_{\mathrm{OL}}(\textbf{r})=\sum_{x,y, x',y'}\epsilon_{1, 2}(\mathrm{cos}^2x+\mathrm{cos}^2y),
$$V_{\mathrm{OL}}(\mathbf{r})=-\frac{V_0}{[1+f(\xi,\eta)]^2}. \eqno{(\textrm{S7})}$$
%\label{OL}
%\end{equation}

%\section*{References}

\end{document}
